# Supplementary material for: A unified framework for multivariate two-sample and k-sample kernel-based quadratic distance goodness-of-fit tests
Source: arXiv:2407.16374 source file (2025-09-30)
Supplement: Supplementary file 1 [file ArXiv_Supplemental.pdf]

# Supplementary Material: A unified framework for Multivariate two-sample and $k$-sample Kernel-based Quadratic Distance Goodness-of-fit tests

Marianthi Markatou*and Giovanni Saraceno

*Department of Biostatistics, University at Buffalo, Buffalo, NY, 14214, USA*

## S1 Two-sample Goodness-of-Fit Tests

The problem of interest is to test the general non parametric hypothesis $H_0 : F = G$ versus the alternative $H_1 : F \neq G$ with $F$ and $G$ unknown. Assume that $\boldsymbol{x}_1, \ldots, \boldsymbol{x}_n$ is a random sample from the distribution of the random variable $\boldsymbol{X} \sim F$ and $\boldsymbol{y}_1, \ldots, \boldsymbol{y}_m$ is a random sample from the distribution of the random variable $\boldsymbol{Y} \sim G$. The corresponding empirical cumulative distribution functions are denoted by $\hat{F}$ and $\hat{G}$. Let $\bar{F}$ be the unknown common distribution under the null hypothesis, i.e. $F = G = \bar{F}$. Then, the kernel-based quadratic distance (KBQD) can be rewritten as

$$\begin{aligned} d_K(F,G) = &\iint K(\boldsymbol{s},\boldsymbol{t})d(F-\bar{F})(\boldsymbol{s})d(F-\bar{F})(\boldsymbol{t}) \\ &- 2\iint K(\boldsymbol{s},\boldsymbol{t})d(F-\bar{F})(\boldsymbol{s})d(G-\bar{F})(\boldsymbol{t}) \\ &+ \iint K(\boldsymbol{s},\boldsymbol{t})d(G-\bar{F})(\boldsymbol{s})d(G-\bar{F})(\boldsymbol{t}). \end{aligned} \tag{1}$$

Centering the kernel $K$ by the distribution $\bar{F}$, we get

$$\begin{aligned} d_K(F,G) = &\iint K_{\bar{F}}(\boldsymbol{s},\boldsymbol{t})dF(\boldsymbol{s})dF(\boldsymbol{t}) \\ &- 2\iint K_{\bar{F}}(\boldsymbol{s},\boldsymbol{t})dF(\boldsymbol{s})dG(\boldsymbol{t}) \\ &+ \iint K_{\bar{F}}(\boldsymbol{s},\boldsymbol{t})dG(\boldsymbol{s})dG(\boldsymbol{t}). \end{aligned}$$

*Corresponding author: markatou@buffalo.edu.

and based on this quantity, the two-sample test statistic is provided as

$$D_{n,m} = \frac{1}{n(n-1)} \sum_{i=1}^{n} \sum_{j\neq i}^{n} K_{\bar{F}}(x_i, x_j) - \frac{2}{nm} \sum_{i=1}^{n} \sum_{j=1}^{m} K_{\bar{F}}(x_i, y_j) \tag{2}$$
$$+ \frac{1}{m(m-1)} \sum_{i=1}^{m} \sum_{j\neq i}^{m} K_{\bar{F}}(y_i, y_j).$$

The cornerstone of the test is the choice of the kernel function, so it should be selected carefully and it must be centered to obtain the asymptotic distribution of the test statistic. In the context of one-sample hypothesis testing, the assumed true distribution $\bar{F}$ under the null hypothesis offers a reasonable guide on the kernel to be used and the appropriate centering distribution. For example, if a $p$-dimensional multivariate normal distribution is assumed under the null hypothesis, we would use the multivariate normal kernel and center it with a multivariate normal distribution with mean and variance matrix estimated from the sample. However, in practice $F$ and $G$ are usually unknown, then we consider a non-parametric centering using

$$\bar{F} = \frac{n}{n+m}\hat{F} + \frac{m}{n+m}\hat{G}.$$

The two-sample test statistic is not modified by the centering distribution, as shown in Lemma 1 of the manuscript. The asymptotic distribution of $D_{n,m}$ under the null hypothesis can be found in Chen [2018].

The two sample test statistic can be derived from the introduced matrix distance

$$\boldsymbol{D} = \begin{pmatrix} D_{11} & D_{12} \\ D_{21} & D_{22} \end{pmatrix} = \begin{pmatrix} \iint K_{\bar{F}}(\boldsymbol{x},\boldsymbol{y})\,dF_1(\boldsymbol{x})\,dF_1(\boldsymbol{y}) & \iint K_{\bar{F}}(\boldsymbol{x},\boldsymbol{y})\,dF_1(\boldsymbol{x})\,dF_2(\boldsymbol{y}) \\ \iint K_{\bar{F}}(\boldsymbol{x},\boldsymbol{y})\,dF_2(\boldsymbol{x})\,dF_1(\boldsymbol{y}) & \iint K_{\bar{F}}(\boldsymbol{x},\boldsymbol{y})\,dF_2(\boldsymbol{x})\,dF_2(\boldsymbol{y}) \end{pmatrix},$$

where $K_{\bar{F}}$ denotes the kernel centered with respect to $\bar{F}$. Then, the covariance matrix of the independent Wishart distribution is given as $\boldsymbol{V} = diag\left(\frac{N}{n}, \frac{N}{m}\right)$, with $N = n + m$.

## S2 Subsample proportion $b$

The non-parametric calculation of the critical value with the subsampling algorithm depends on the subsample size $n_B = n{*}b$, with $b \in (0, 1]$. We investigate the performance of the proposed KBQD tests using the subsampling algorithm with respect to different values of $b$, when $k = 2$. In particular, we consider $b = 0.3, 0.5, 0.8$. We generated samples $\boldsymbol{x}_1, \ldots, \boldsymbol{x}_{n_1}$ from the normal distribution $N_d(\boldsymbol{0}, \boldsymbol{I}_d)$ and $\boldsymbol{y}_1, \ldots, \boldsymbol{y}_{n_2}$ from the skew-normal distribution $SN_d(\boldsymbol{0}, \boldsymbol{I}_d, \boldsymbol{\lambda})$, where $\boldsymbol{I}_d$ denotes the $d$-dimensional identity matrix, $\boldsymbol{\lambda} = \lambda\boldsymbol{1}$ and $\lambda = 0, 0.1, 0.2, 0.3$. Observations are sampled using the `R` package `sn`. We considered dimensions $d = 1, 2, 6$, sample size $n_1 = n_2 = 1000, 3000, 5000$ and $N = 500$ replications. The KBQD test is computed for $h = 0.2(0.4)10$ and $B = 150$.

Figure S1 shows the boxplots of critical values computed with the subsampling algorithm for $h = 2.2$ and different values of $n$ and $d$, indicated as headers. The computed

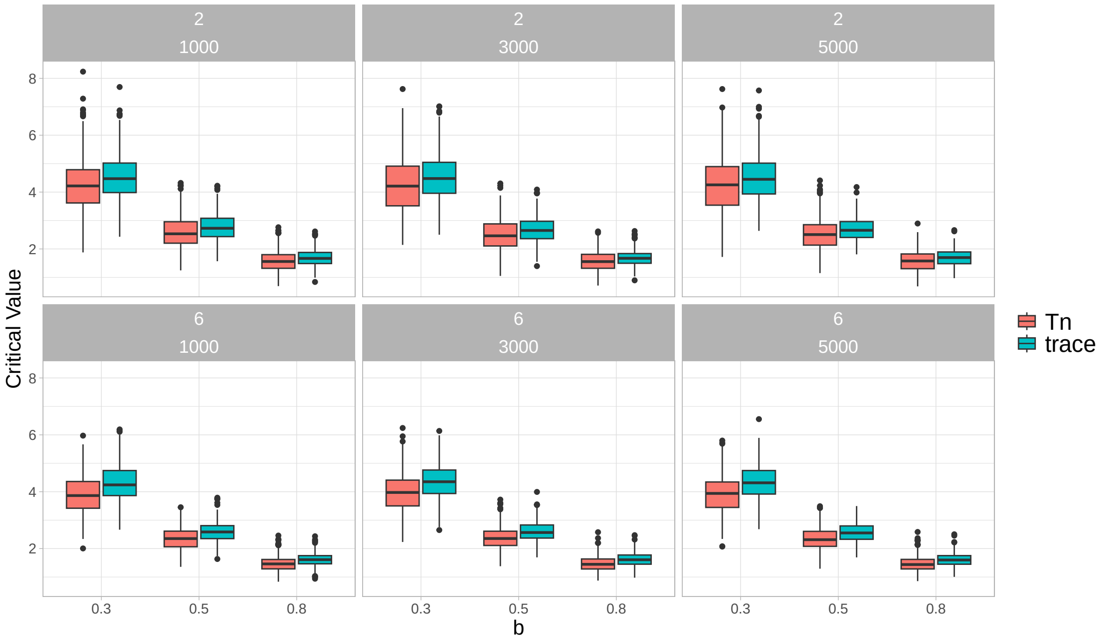


**Fig. S1** Boxplots of critical values of the KBQD test statistics, $T_n$ and trace, for increasing subsample proportion $b$ with respect to the subsampling algorithm, and dimension $d = 2, 6$ and sample size $n = 1000, 3000, 5000$, indicated as headers. $h = 2.2$ and $\lambda = 0$.

critical values are larger for smaller proportion $b$. Then, we investigate if the KBQD tests are affected by the value of $b$, in terms of level and power. Figure S2 shows the performance of the KBQD tests with respect to $b$, for increasing $h$, in terms of level (top), with dimension $d = 2, 6$ and sample size $n$ indicated as header, and power (bottom) with $\lambda = 0.1, 0.2, 0.3$ and $n$, indicated as headers and $d = 6$. In general, subsampling with lower proportion $b$ achieves a lower level than the nominal level. In terms of power, decreasing the proportion $b$ the KBQD test achieves lower power only for low sample size and for alternatives close to the null hypothesis. Figure S3 illustrates the power of the KBQD tests for the subsampling algorithm across different values of $b$ for increasing skewness $\lambda$, when $n = 1000, 3000, 5000$, $d = 1, 2, 6$. For smaller sample size and dimension, the test with a smaller proportion $b$ achieves lower power, while for the other combinations of parameter values the obtained power does not change significantly. In summary, for large sample sizes, a smaller proportion, for example $b = 0.5$, can be considered optimal since it achieves high power with minimal loss in level performance and significantly reduces computational time. Based on the evaluation of the performance of the KBQD tests with respect to the proportion $b$ reported in this section, we recommend using $b = .8$ as default setting, while suggesting lower value as the sample size increases.

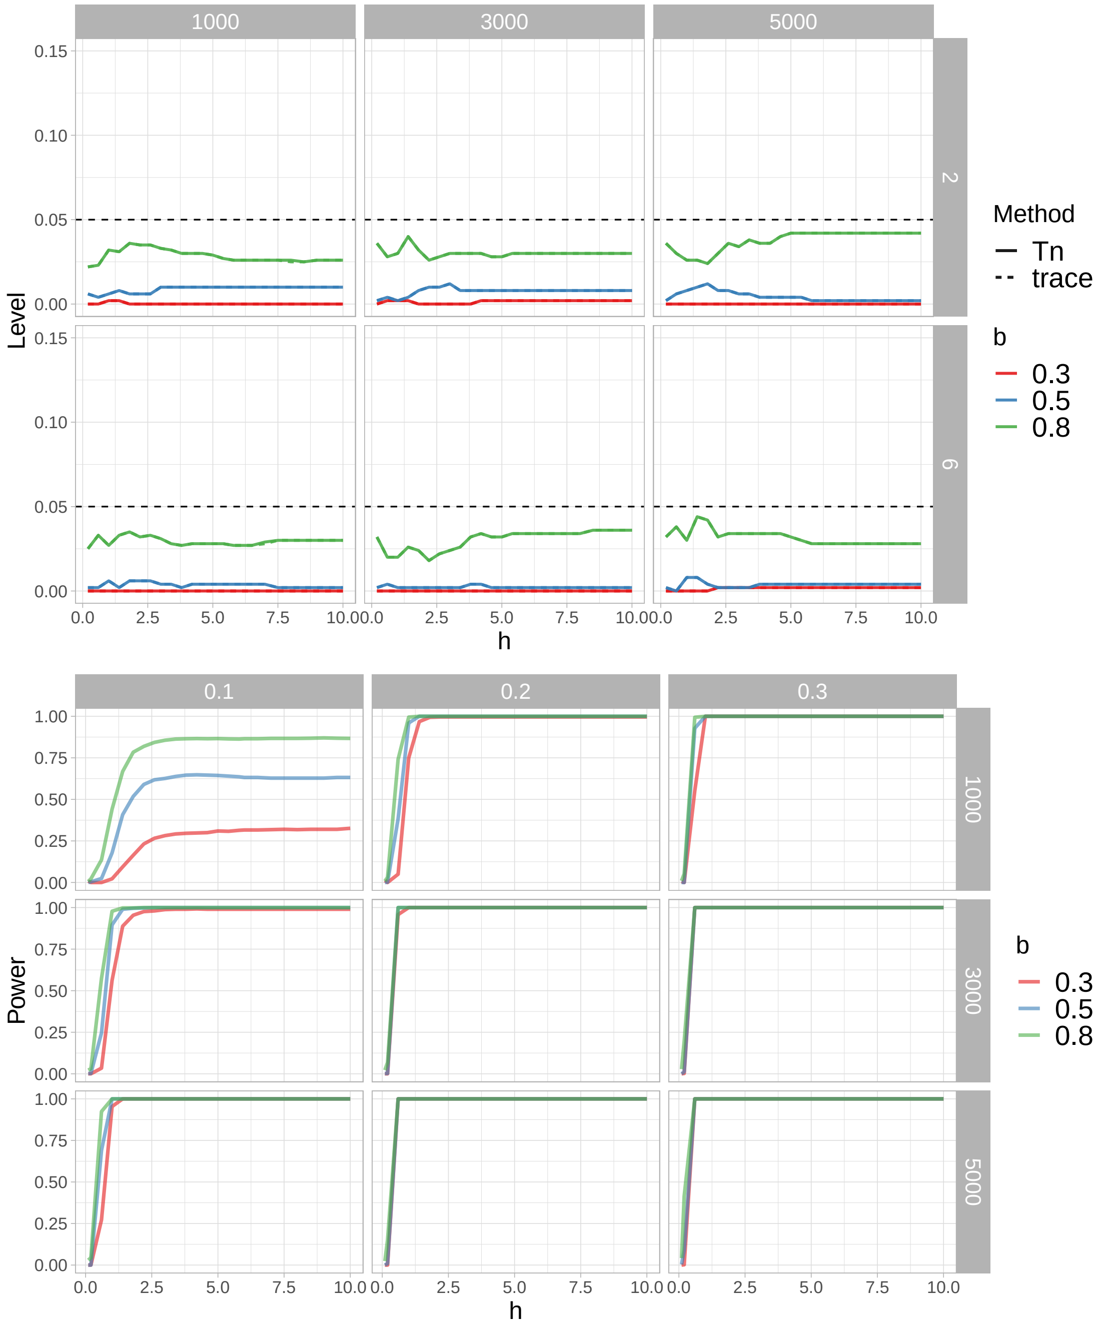


**Fig. S2** (top) Level of KBQD tests for increasing $h$ with respect to the subsampling algorithm for different $b$, with $n = 1000, 3000, 5000$ and $d = 2, 6$. The dashed line denotes the nominal level $\alpha = 0.05$. (bottom) Power of KBQD tests for increasing $h$, with $n = 1000, 3000, 5000$ and $\lambda = 0.1, 0.2, 0.3$ indicated as headers, and $d = 6$.

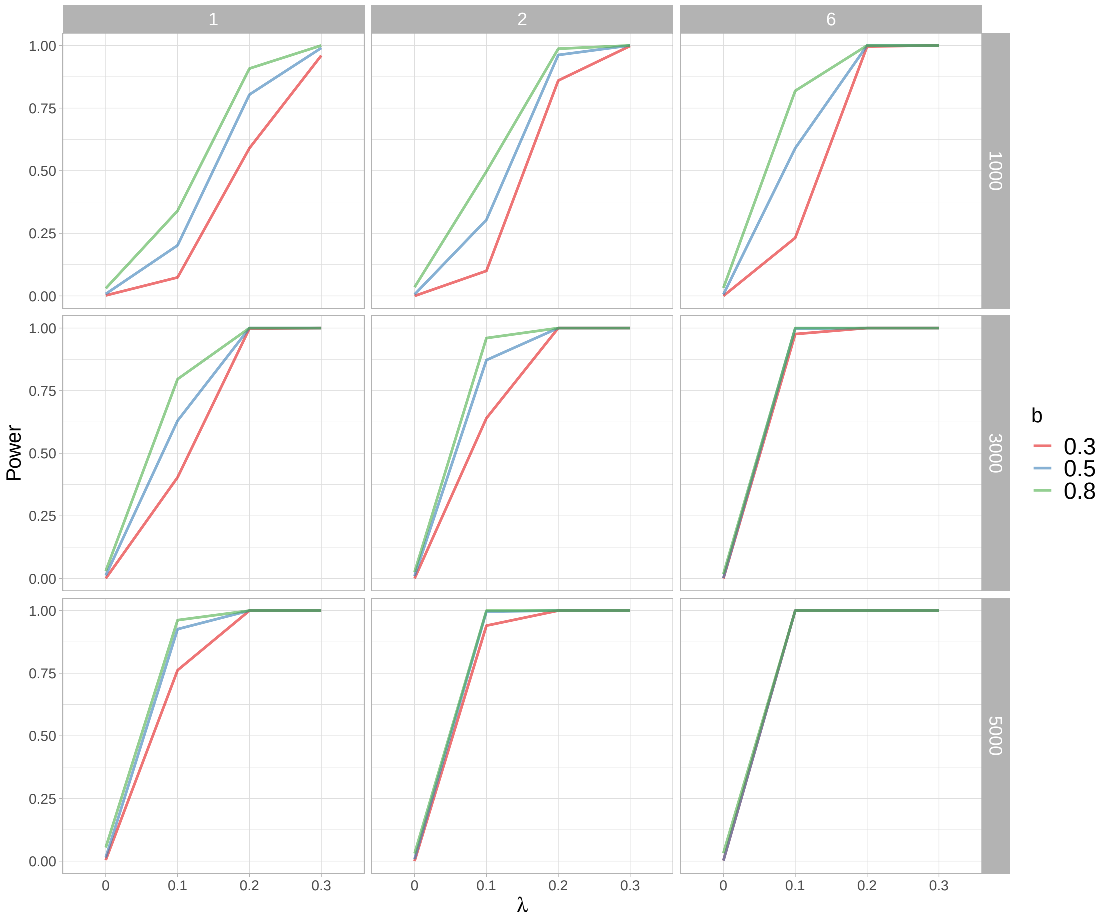


**Fig. S3** Power of KBQD tests for increasing $h$ with respect to the bootstrap, permutation and subsampling algorithm, for $n = 100, 500$, $N = 1000$ replications, $d = 6$ and $\lambda = 0.3$.

## S3 Computation of the critical value

In this section, we show additional results regarding the simulation study for the computation of the critical value of the two-sample test statistic with respect the number of replications $B$, introduced in Section 4 of the manuscript. Figure S4 displays the boxplots of the critical values of the KBQD two-sample test with respect to $h$, for sample size $n = 100, 500, 1000$ indicated as header and $d = 2$ (top) for dimension $d = 1, 2, 6$ indicated as header and $n = 500$ (bottom) . The distribution of the computed critical values does not show significant differences with respect to the considered sample sizes, dimensions and values of $h$. Figure S5 shows the boxplots of the critical values with respect to $\lambda$, for the bootstrap, permutation and subsampling algorithms, with $B = 150$, $d = 1, 2, 6$ and $n = 100, 500, 1000$ for completeness.

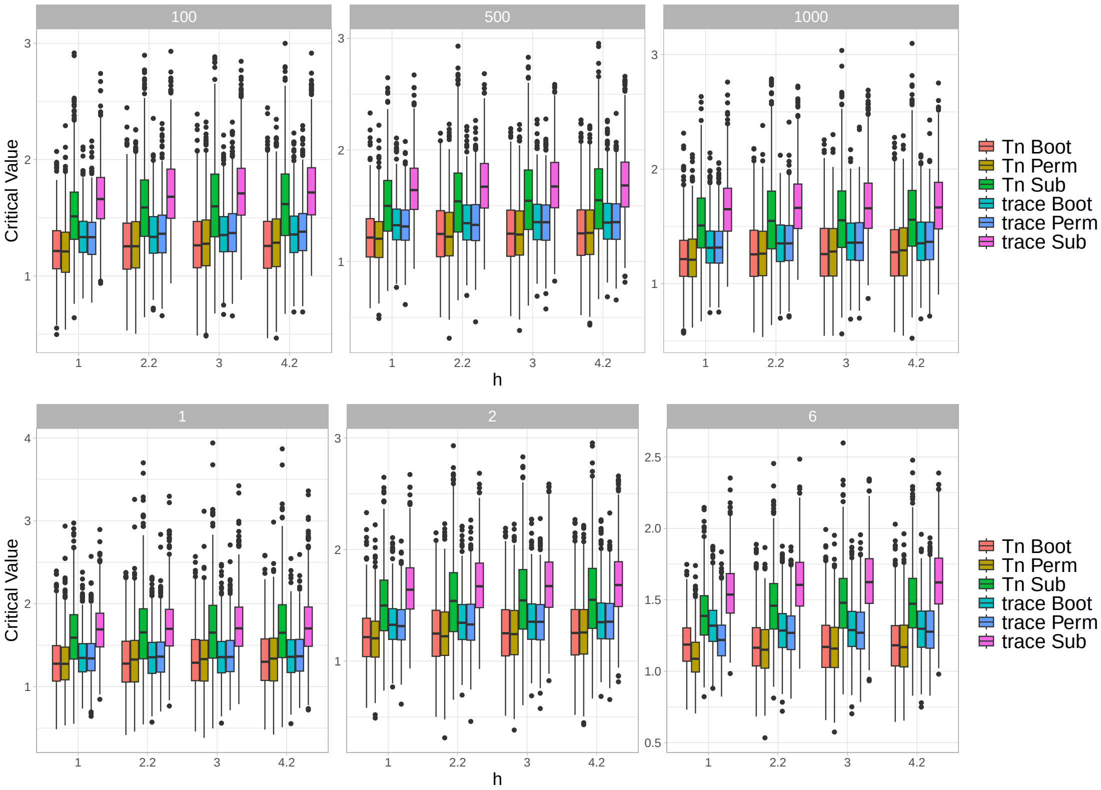


**Fig. S4** Boxplots of critical values of KBQD tests for different values of the tuning parameter $h = 1, 2.2, 3, 4.2$ on the $x$-axis, with respect to the bootstrap, permutation and subsampling algorithm, $B = 150$ and $\lambda = 0$. (top) The sample size $n = 100, 500, 1000$ is indicated as header, and $d = 2$. (bottom) The dimension $d = 1, 2, 6$ is indicated as header, and $n = 500$.

# S4 Other asymmetric distributions

In this section, we provide additional simulation results considering other families of asymmetric alternatives. In particular, we generate samples from the univariate Gumbel distribution Gumbel$(\mu, \sigma)$, using the function `rgumbel` in the `R` package `evd`, and the univariate log-normal distribution $\log -N(\mu, \sigma)$ using the function `rlnorm` in the `R` package `stats`, both depending on two parameters. The following simulation scenarios are investigated.

(i) $X \sim \log{-N}(0, 0.8)$ and $Y \sim \log -N(0, \sigma)$, where $\sigma = 0.6, 0.65, 0.7, 0.75, 0.8$.

(ii) $X \sim$ Gumbel$(0, 1)$ and $Y \sim$ Gumbel$(\mu, 1)$, where $\mu = 0, 0.1, 0.2, 0.3$.

(iii) $X \sim$ Gumbel$(0, 1)$ and $Y \sim$ Gumbel$(0, \sigma)$, where $\sigma = 0.8, 0.9, 1, 1.1, 1.2$.

The considered families of alternatives are displayed in Figure S6 and Figure S7, respectively. For each scenario, we consider sample size $n = m = 100, 500, 1000$ and number of

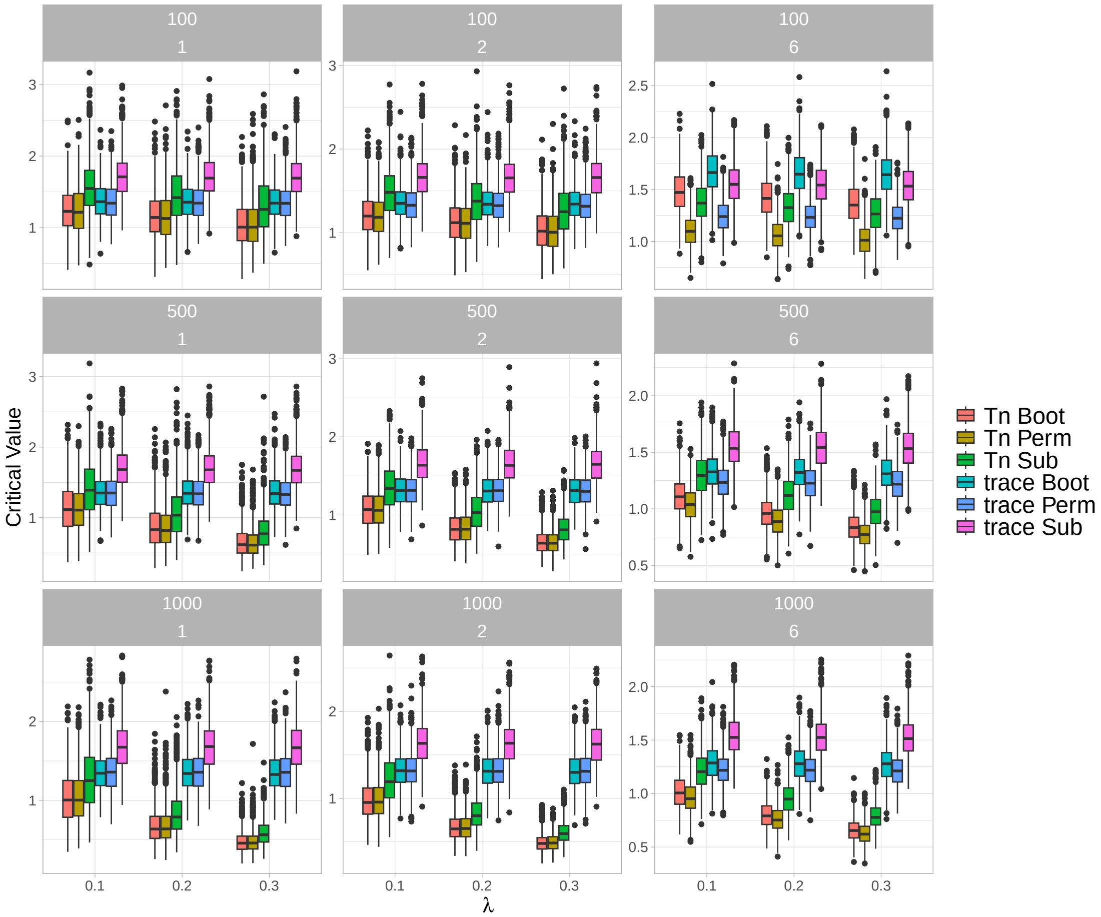


**Fig. S5** Boxplots of critical values of the KBQD test for increasing $\lambda$ with respect to the bootstrap, permutation and subsampling algorithm, for different values of dimension $d$ and sample size $n$, indicated as header of $x$-axis and $y$-axis, respectively. KBQD tests are combute for $B = 150$ and $h = 1$.

replications $N = 100$. For the selection of the tuning parameter $h$, we consider different values, that is $h = 0.2(0.4)10$. The smallest value of $h$ which yields power greater or equal to 0.5 is selected as optimal, according to the procedure described in algorithm 2 of the main manuscript.

Figure S8, Figure S10 and Figure S12 show the performance of the proposed kernel-based tests, using the bootstrap, permutation and subsampling algorithms, with respect to the tuning parameter $h$ for the described scenarios. When the alternative distribution is close to the null hypothesis, the choice of $h$ does not affect the power of the resulting test. When the departure from the null hypothesis is more evident, a range of values is suggested for obtaining powerful tests. In particular, for the scenario $(ii)$, the simulation results suggest that all the values greater than a certain threshold can be chosen for opti-

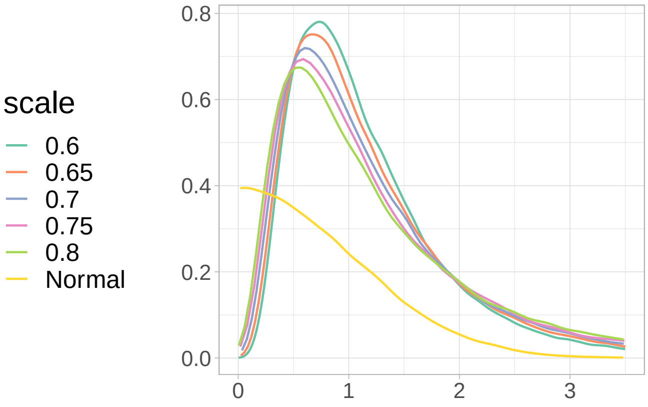


**Fig. S6** Kernel density estimates of univariate log $-N(\mu, \sigma)$ distribution with $\sigma = 1$ and different values of $\mu$.

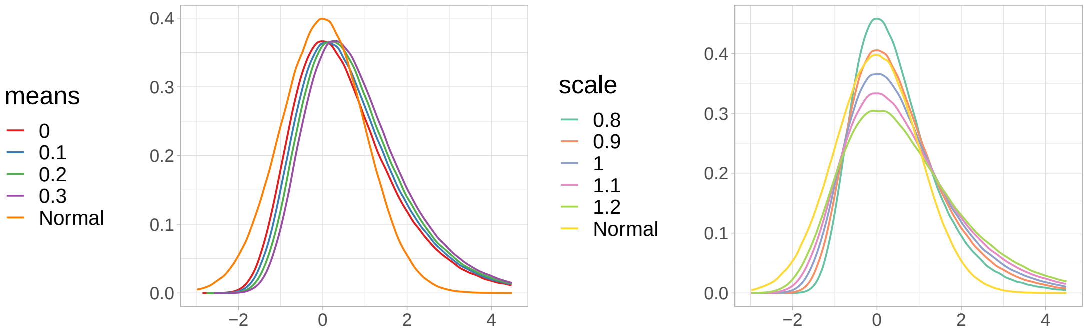


**Fig. S7** (left) Kernel density estimates of univariate Gumbel$(\mu, 1)$ distribution with different values of $\mu$. (right) Kernel density estimates of univariate Gumbel$(0, \sigma)$ distribution with different values of $\sigma$.

mal power (Figure S10), while for the other two scenarios the optimal choices reduce to a smaller interval (Figure S8 and Figure S12), indeed for increasing $h$ the power decreases.

Figure S9 shows the performance in terms of power of the KBQD tests in comparison to the MMD and energy tests, when the log-normal distribution is considered. Figure S11 and Figure S13 display the achieved power of the considered two-sample tests when the family of alternatives follows the Gumbel distribution, according to scenarios $(ii)$ and $(iii)$, respectively. The KBQD tests show an improved power with respect to MMD and energy tests, especially for low sample size. The two kernel-based tests achieve the same performance for increasing sample size and departure from the null hypothesis.

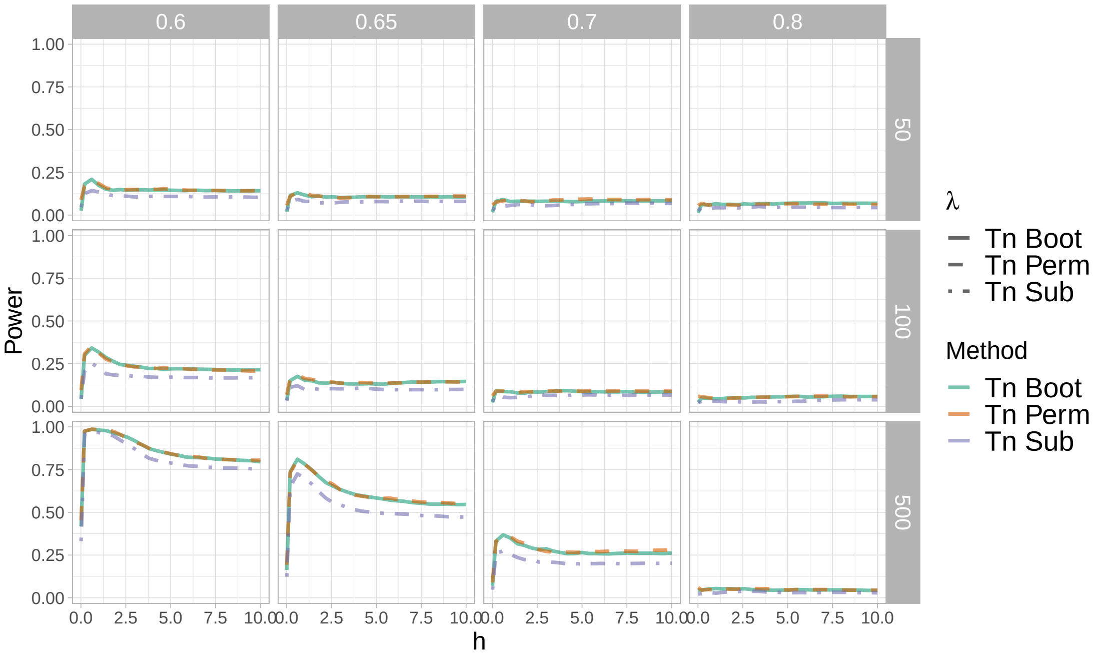


**Fig. S8** Power of the kernel-based tests, computed using the bootstrap, permutation and subsampling algorithm, with respect to the parameter $h$ for samples generated from $\log N(0, \sigma)$ distribution for different values of $\sigma$ and samples size.

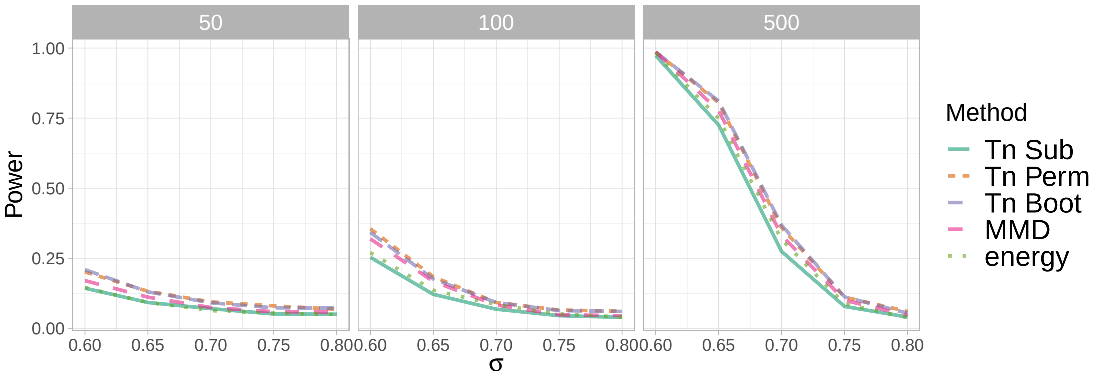


**Fig. S9** Power of the considered tests with respect for samples generated from $\log\mathrm{N}(0, \sigma)$ distribution for different values of $\sigma$ and samples size. The null hypothesis states that the distribution is $\log\mathrm{N}(0, 0.8)$.

# S5 Additional simulation results

In this section we show additional results for the simulation scenarios presented in section 5 of the main paper.

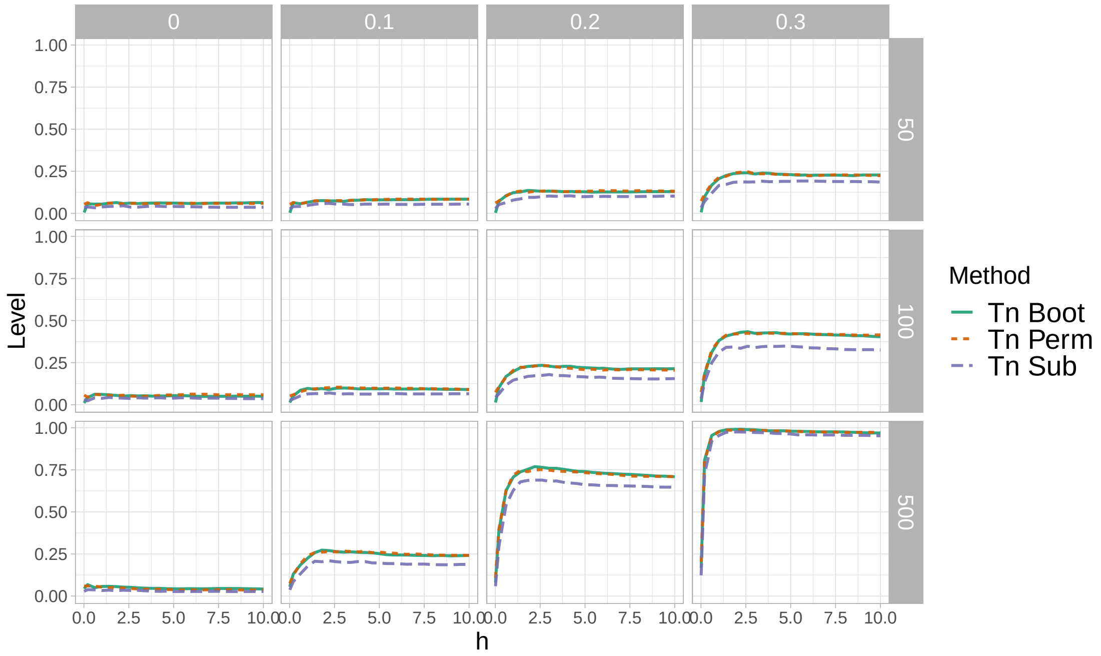


**Fig. S10** Power of the kernel-based tests, computed using the bootstrap, permutation and subsampling algorithm, with respect to the parameter $h$ for samples generated from Gumbel$(\mu, 1)$ distribution for different values of $\mu$ and samples size.

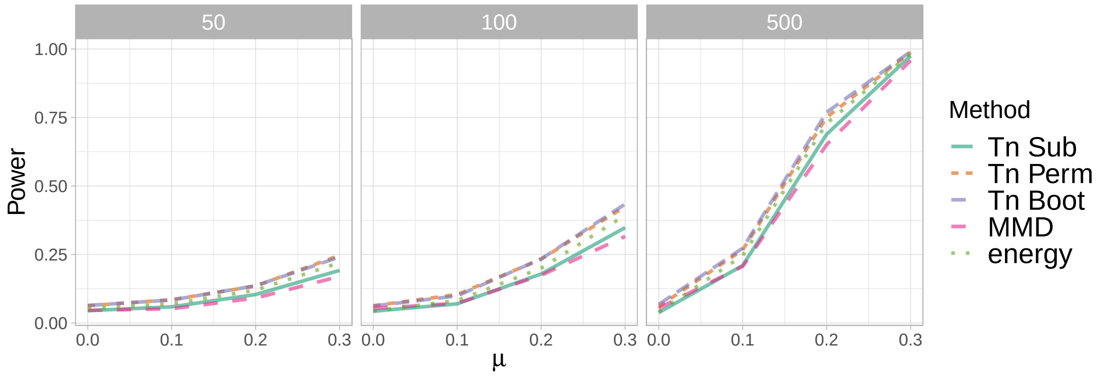


**Fig. S11** Power of the considered tests with respect for samples generated from Gumbel$(\mu, 1)$ distribution for different values of $\mu$ and samples size. The null hypothesis states that the distribution is Gumbel$(0, 1)$.

## S5.1 Scenario 1

For completeness, Figure S14 illustrates the level of the KBQD two-sample tests as a function of the tuning parameter $h$, using the three different sampling methods to calculate the empirical critical value. The horizontal line in these plots indicates the

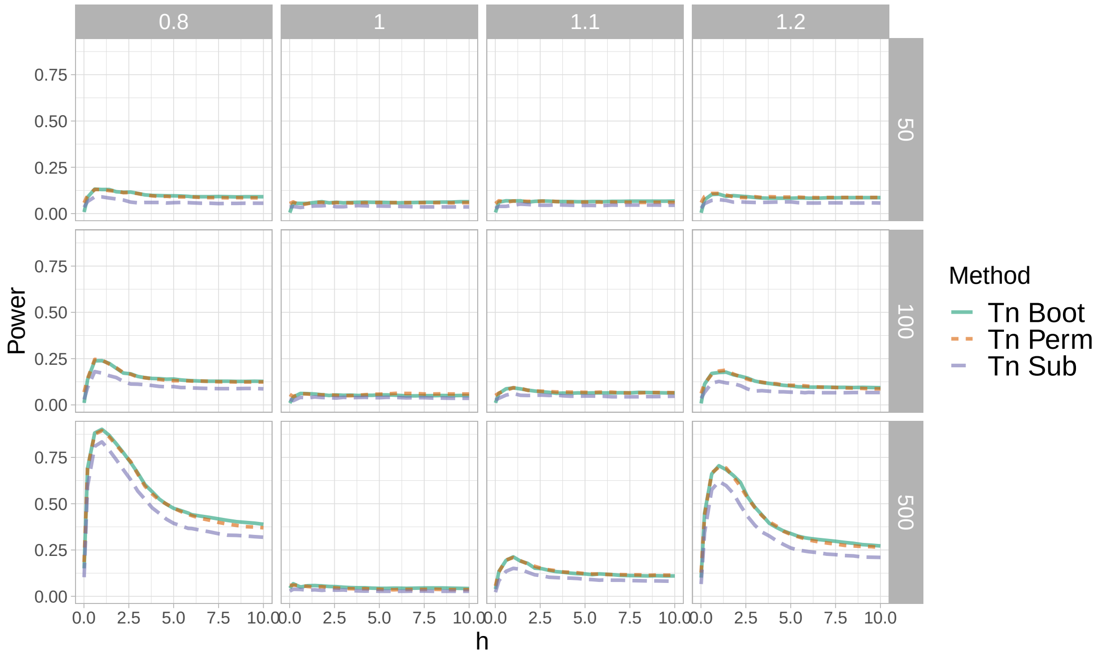


**Fig. S12** Power of the kernel-based tests, computed using the bootstrap, permutation and subsampling algorithm, with respect to the parameter $h$ for samples generated from Gumbel$(0, \sigma)$ distribution for different values of $\sigma$ and samples size.

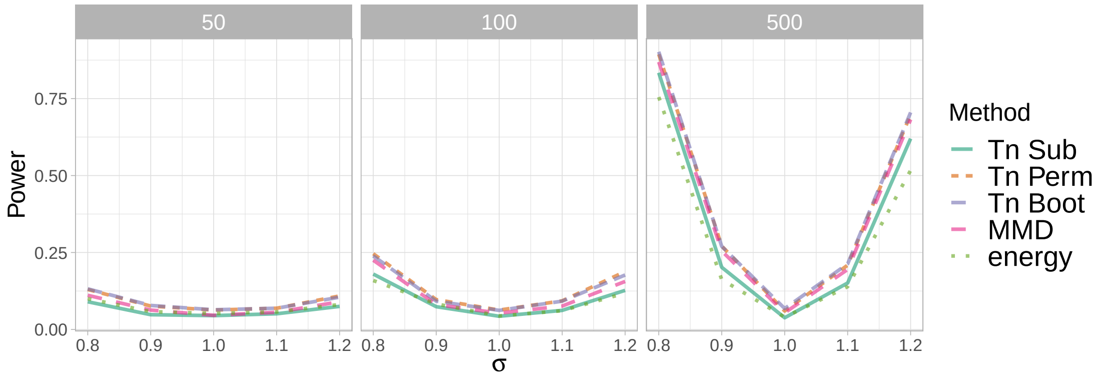


**Fig. S13** Power of the considered tests with respect for samples generated from Gumbel$(0, \sigma)$ distribution for different values of $\sigma$ and samples size. The null hypothesis states that the distribution is Gumbel$(0, 1)$.

theoretical level $\alpha = 0.05$. Figure S15 shows the power of the proposed tests as a function of the tuning parameter $h$ for different values of the skewness parameter $\lambda$, $d = 1$ and $n = 500, 1000$. We next compare the performance of the KBQD test against the existing multivariate two-sample goodness-of-fit tests. In Figure S16, we compare

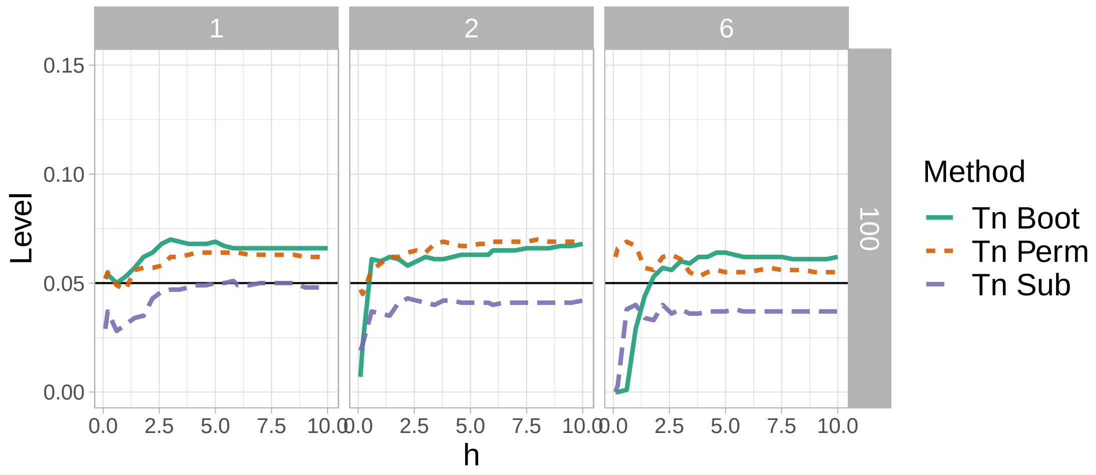


**Fig. S14** Scenario 1: Level of KBQD $T_n$, with critical value computed using Bootstrap, Permutation and Subsampling, as function of the tuning parameter $h$, for the combinations of dimension $d = 1, 2, 6$ and sample size $n = 100$, indicated as headers.

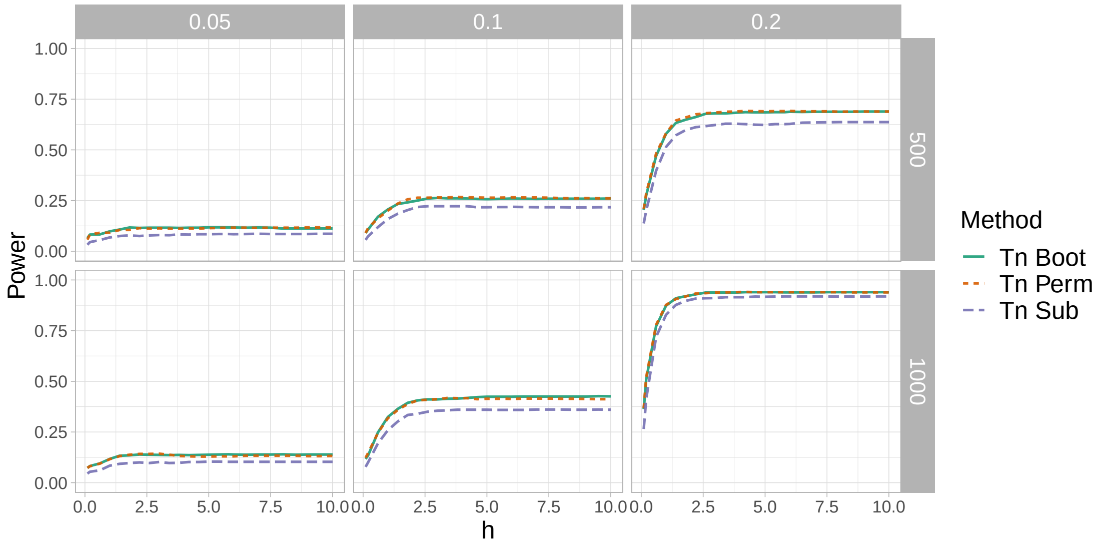


**Fig. S15** Scenario 1: Power of KBQD test $T_n$, with the critical value computed using bootstrap, permutation and subsampling, as function of $h$. $\lambda = 0.05, 0.1, 0.2$, $d = 1$ and $n = 500, 1000$.

the level of the considered two-sample tests with respect to the sample size $n$ and the dimension $d$. Figure S17 illustrates the power of the proposed KBQD tests in comparison with the competitor two-sample tests, with respect to the skewness parameter $\lambda$, for different dimensions and sample sizes, indicated as headers. The tuning parameter of the KBQD tests is obtained via the use of algorithm 2. The Crossmatch, FR-WW and

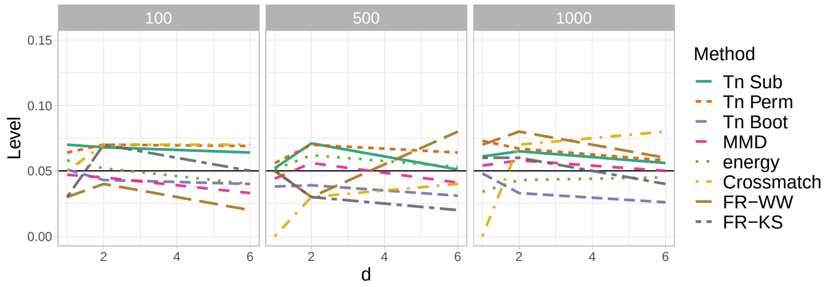


**Fig. S16** Scenario 1: Level of KBQD tests, with critical value computed using Bootstrap, Permutation and Subsampling, compared to the considered two-sample tests with respect to the dimension $d$ and sample size $n$ indicated as header. The tuning parameter of the KBQD tests is obtained via algorithm 2.

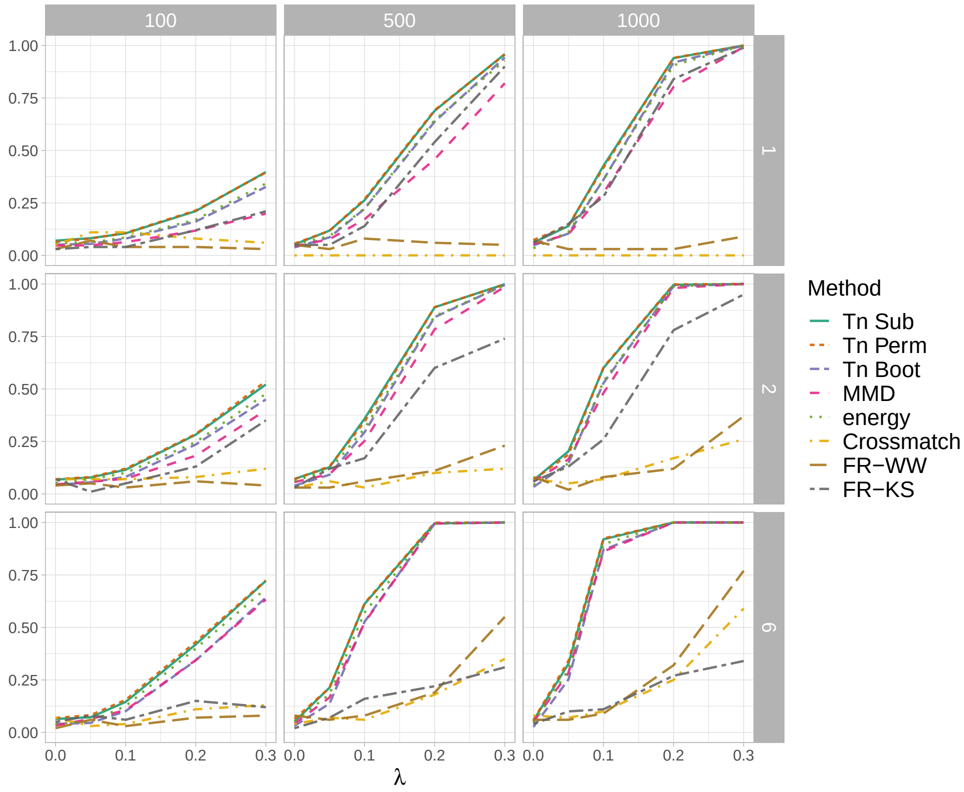


**Fig. S17** Scenario 1: Power of KBQD test $T_n$, with the critical value computed using bootstrap, permutation and subsampling, compared with the considered two-sample tests as function of $\lambda$ for sample size $n$ and dimension $d$, indicated as headers on the $x$-axis and $y$-axis respectively. The tuning parameter of the KBQD tests is obtained via algorithm 2.

FR-KS two-sample tests exhibit a poor performance against asymmetric alternatives, with the exception of the FR-KS which is competitive in the univariate case. KBQD tests are, the MMD and energy test are competitive and outperform the remaining tests.

## S5.2 Scenario 2

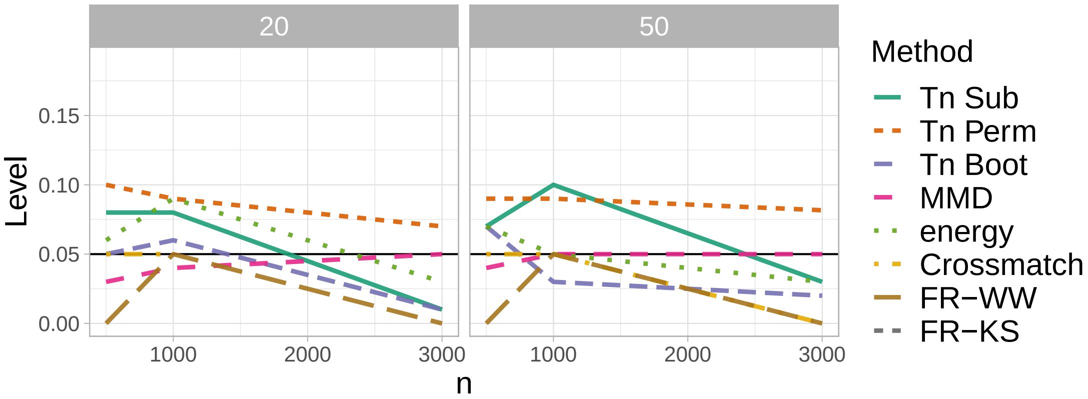


**Fig. S18** Scenario 2: Level of KBQD test $T_n$, with the critical value computed using bootstrap, permutation and subsampling, compared with the considered two-sample tests, for dimension $d = 20, 50$ and sample size $n = 500, 1000, 3000$. The tuning parameter of the KBQD tests is obtained via algorithm 2.

Figure S18 illustrates the level of the proposed KBQD test $T_n$ in comparison to the considered two-sample tests, for increasing $n$ and dimension $d = 20, 50$. Figure S19 shows the power of the proposed KBQD test $T_n$ in comparison to the considered two-sample tests, with respect to the skewness parameter $\lambda$, for dimension $d$ and sample size $n$ indicated as headers. The Crossmatch, FR-WW and FR-KS tests have a poor performance in terms of both level and power.

## S5.3 Scenario 3

We present the simulation results for Scenario 3 presented in section 5 of the main paper. We start measuring the performance of the KBQD tests in terms of achieved level. Figure S20 illustrates the level of the KBQD two-sample tests as a function of the tuning parameter $h$, using the bootstrap, permutation and subsampling algorithm to calculate the empirical critical value. The horizontal line in these plots indicates the theoretical level $\alpha = 0.05$. Figure S21 shows the power of the proposed tests as a function of the tuning parameter $h$ for different values of the skewness parameter $\lambda$, $d = 7$ and $n = 100, 500$. We next compare the performance of the KBQD test with the existing multivariate two-sample goodness-of-fit tests. In Figure S22, we compare the level of the considered two-sample tests with respect to the sample size $n$ and the dimension $d$. Figure S23 illustrates the power of the proposed KBQD tests in comparison

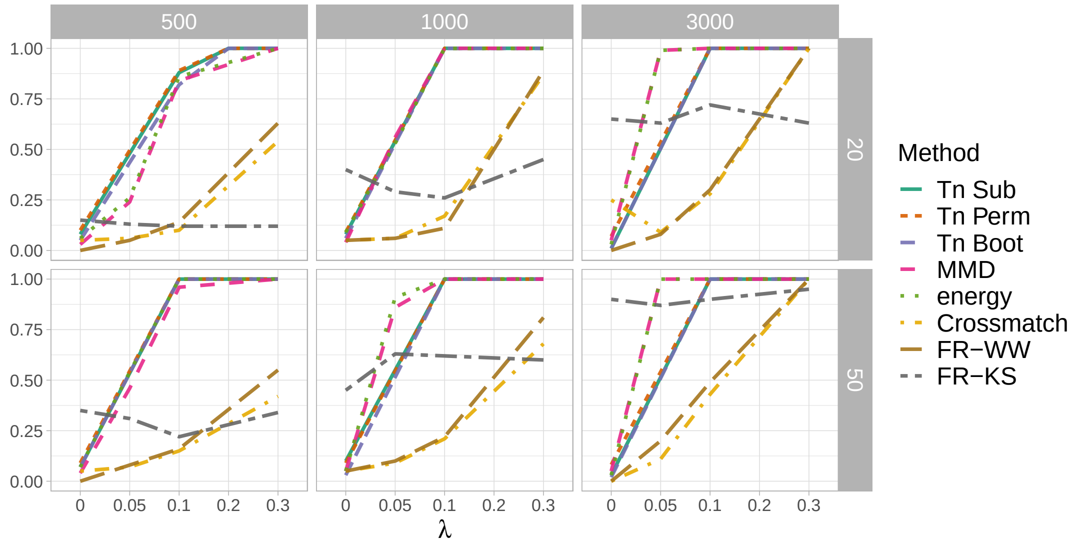


**Fig. S19** Scenario 2: Power of KBQD test $T_n$, with the critical value computed using bootstrap, permutation and subsampling, compared with the considered two-sample tests, for dimension $d = 20, 50$ and sample size $n = 500, 1000, 3000$ indicated as headers. The tuning parameter of the KBQD tests is obtained via algorithm 2.

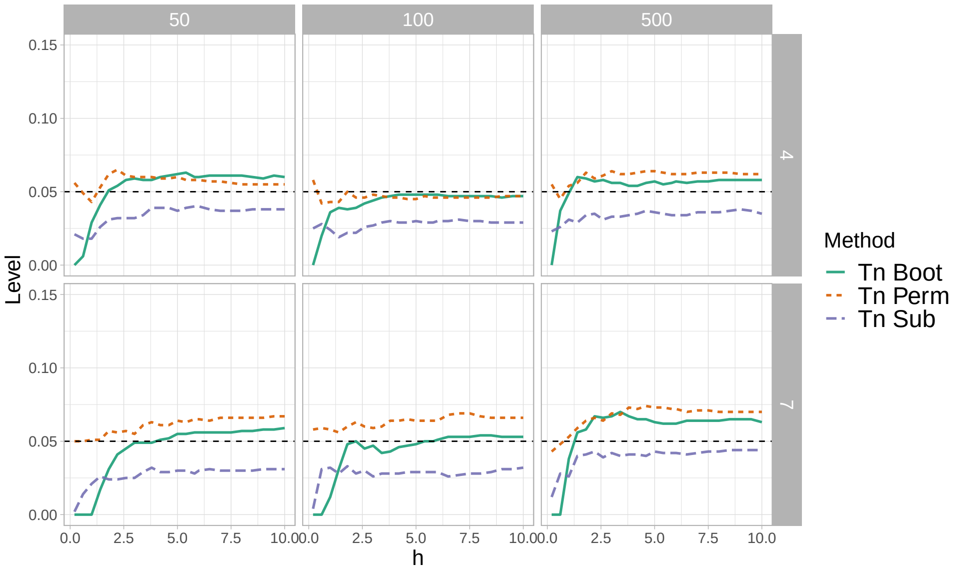


**Fig. S20** Scenario 3: Level of KBQD $T_n$, with critical value computed using Bootstrap, Permutation and Subsampling, as function of the tuning parameter $h$, for the combinations of dimension $d = 4, 7$ and sample size $n = 50, 100, 500$, indicated as headers.

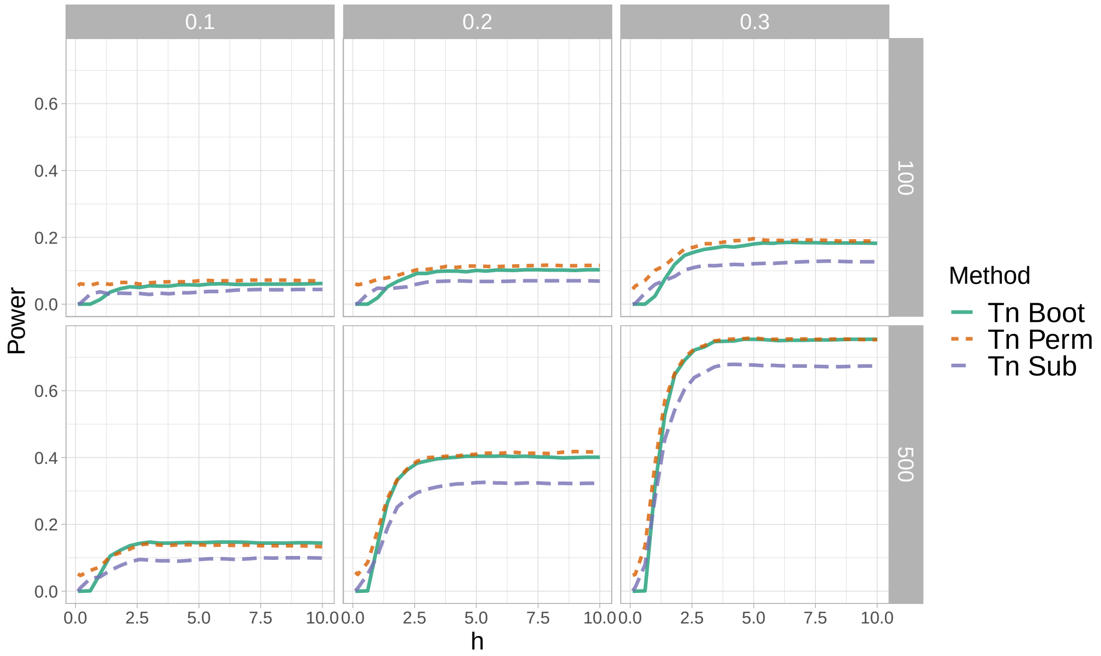


**Fig. S21** Scenario 3: Power of KBQD test $T_n$, with the critical value computed using bootstrap, permutation and subsampling, as function of $h$. $\lambda = 0.1, 0.2, 0.3$, $d = 7$ and $n = 100, 500$.

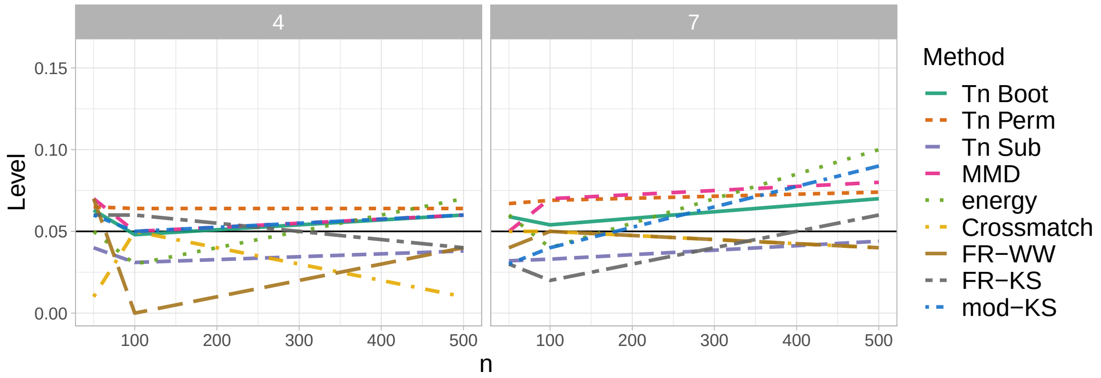


**Fig. S22** Scenario 3: Level of KBQD test $T_n$, with the critical value computed using bootstrap, permutation and subsampling, compared with the considered two-sample tests, for dimension $d = 4, 7$ and sample size $n = 50, 100, 500$. The tuning parameter of the KBQD tests is obtained via algorithm 2.

with the competitor two-sample tests, with respect to the skewness parameter $\lambda$, for different dimensions and sample sizes, indicated as headers. The tuning parameter of the tests is obtained via the use of algorithm 2. The KBQD tests consistently demonstrate

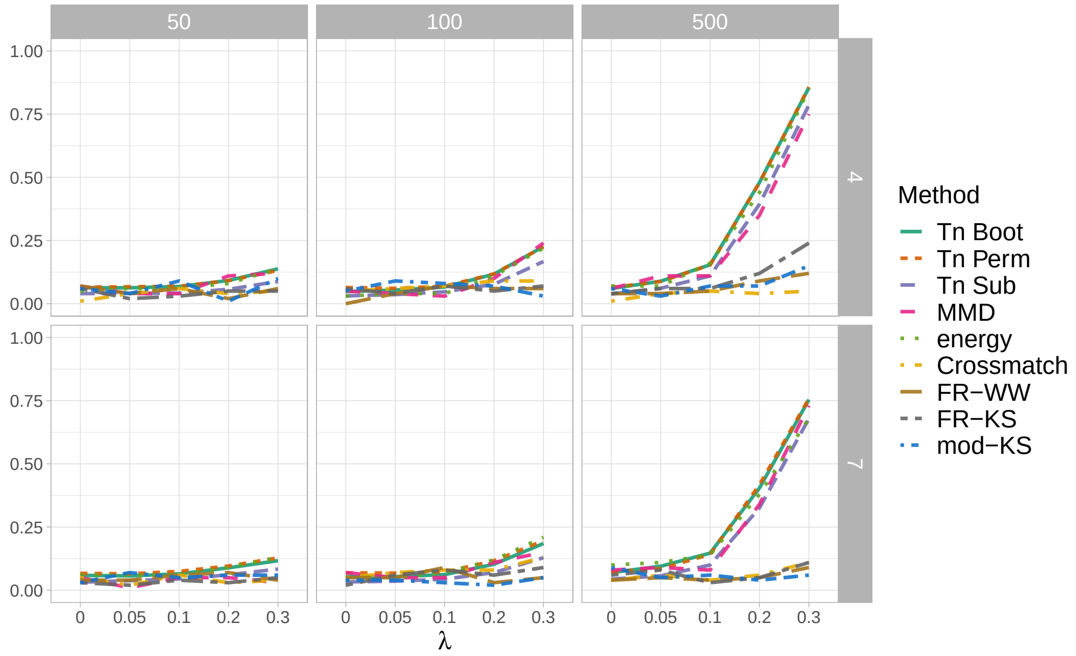


**Fig. S23** Scenario 3: Power of KBQD test $T_n$, with the critical value computed using bootstrap, permutation and subsampling, compared with the considered two-sample tests, for dimension $d = 4, 7$ and sample size $n = 50, 100, 500$ indicated as headers. The tuning parameter of the KBQD tests is obtained via algorithm 2.

enhanced power performance compared to the other tests, especially when the sample size increases. The Crossmatch, FR-WW and FR-KS two-sample tests exhibit a poor performance.

## S5.4 $t$-distribution

We report here the simulation results for alternatives following the $t$-distribution. Figure S24 depicts the level obtained by the KBQD tests, the energy test and the independence tests when testing the equality of samples from $t$-distributions as function of the sample size $n$, for different values of dimension $d$ and number of samples $K$. Figures S25 and S26 compare the performance of the $k$-sample tests in terms of power as function of $\varepsilon$, with **Type 1** and **Type 2** alternatives, for $K = 3$ and $k = 5$ samples, respectively. Different combinations of dimension $d$ and sample size (per sample) $n$ are displayed. The KBQD tests with the bootstrap and permutation algorithms show slightly higher level than the nominal one. On the other hand, using the subsampling algorithm, the level is lower, still close to the nominal level. In terms of power, the considered tests perform similarly.

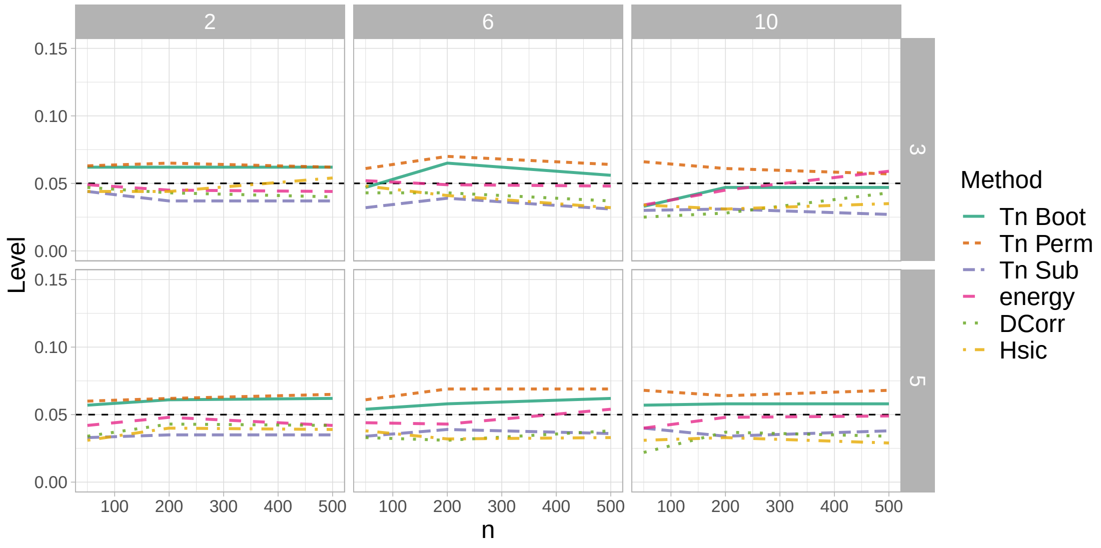


**Fig. S24** $t$-distribution: Level of KBQD test $T_n$, with the critical value computed using bootstrap, permutation and subsampling, for increasing sample size $n$ compared with the listed $k$-sample tests, for dimension $d = 2, 6, 10$ and number of samples $K = 3, 5$ indicated as headers. The tuning parameter of the KBQD tests is obtained via algorithm 2.

# S6 Penguin data set

In this section, we report some additional details regarding the Penguin data set application. Table S1 shows a summary of the variables in the Penguin dataset. The categorical variable "Island" is summarized as relative percentages and absolute counts, while the remaining variables with mean and standard deviation (SD), median and interquantile range, minimum and maximum, and skewness, computed by group and overall. Finally, Table S2 reports the test statistics, critical values or $p$-values for the performed $k$-sample tests, with $k = 3$. All the considered tests reject the equality of the distributions from the three groups.

# References

Yang Chen. *Contribution to the Theory and Application of Statistical Distances.* Phd thesis, University at Buffalo, Department of Biostatistics, Buffalo, NY, 2018.

Table S1: Summary of variables in the Penguin dataset overall and with respect to the species.

| | Adelie (n=151) | Chinstrap (n=68) | Gentoo (n=123) | Overall (n=342) |
|---|---|---|---|---|
| **Island** | | | | |
| Biscoe | 44 (29.1%) | 0 (0%) | 123 (100%) | 167 (48.8%) |
| Dream | 56 (37.1%) | 68 (100%) | 0 (0%) | 124 (36.3%) |
| Torgersen | 51 (33.8%) | 0 (0%) | 0 (0%) | 51 (14.9%) |
| **bill length (mm)** | | | | |
| Mean (SD) | 38.8 (2.66) | 48.8 (3.34) | 47.5 (3.08) | 43.9 (5.46) |
| Median [IQR] | 38.8 [4.00] | 49.6 [4.73] | 47.3 [4.25] | 44.5 [9.28] |
| Min - Max | 32.1 - 46.0 | 40.9 - 58.0 | 40.9 - 59.6 | 32.1 - 59.6 |
| Skewness | 0.16 | -0.089 | 0.643 | 0.053 |
| **bill depth (mm)** | | | | |
| Mean (SD) | 18.3 (1.22) | 18.4 (1.14) | 15.0 (0.981) | 17.2 (1.97) |
| Median [IQR] | 18.4 [1.50] | 18.5 [1.90] | 15.0 [1.50] | 17.3 [3.10] |
| Min - Max | 15.5 - 21.5 | 16.4 - 20.8 | 13.1 - 17.3 | 13.1 - 21.5 |
| Skewness | 0.318 | 0.007 | 0.32 | -0.143 |
| **flipper length (mm)** | | | | |
| Mean (SD) | 190 (6.54) | 196 (7.13) | 217 (6.84) | 201 (14.1) |
| Median [IQR] | 190 [9.00] | 196 [10.0] | 216 [9.00] | 197 [23.0] |
| Min - Max | 172 - 210 | 178 - 212 | 203 - 231 | 172 - 231 |
| Skewness | 0.086 | -0.009 | 0.39 | 0.344 |
| **body mass (g)** | | | | |
| Mean (SD) | 3700 (459) | 3730 (384) | 5080 (504) | 4200 (802) |
| Median [IQR] | 3700 [650] | 3700 [463] | 5000 [800] | 4050 [1200] |
| Min - Max | 2850 - 4780 | 2700 - 4800 | 3950 - 6300 | 2700 - 6300 |
| Skewness | 0.282 | 0.242 | 0.069 | 0.468 |

Table S2: Results of the considered $k$-sample tests when comparing the three species in the Penguin data set. For each test, the obtained test statistic, the critical value or the $p$-value, and the final answer to the null hypothesis are displayed. The value of $h$ is selected via algorithm 2.

| Method | $h$ | Statistics | critical Value | p-value | reject $H0$ |
|---|---|---|---|---|---|
| Tn Sub | 1.6 | 3.976631 | 0.8563107 | - | TRUE |
| Tn Boot | 1.2 | 3.10071 | 3.034766 | - | TRUE |
| Tn Perm | 1.2 | 3.10071 | 0.6986339 | - | TRUE |
| energy | - | 114226 | - | 0.006623 | TRUE |
| Dcorr | - | 0.54185 | - | 2.029855e-42 | TRUE |
| Hsic | - | 0.54185 | - | 2.029855e-42 | TRUE |

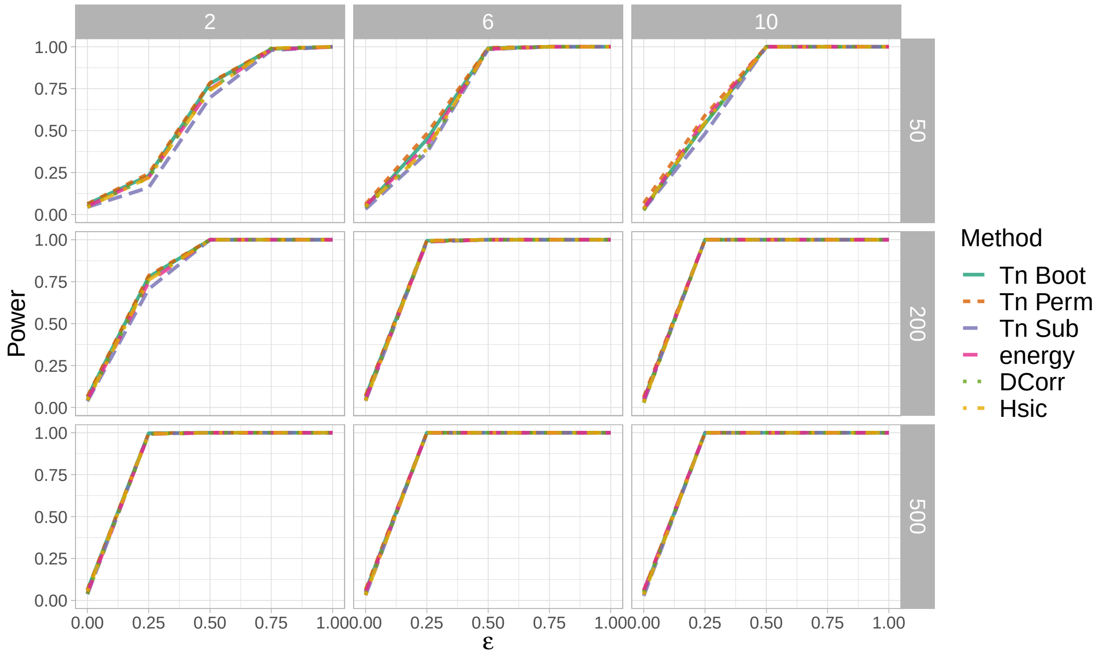


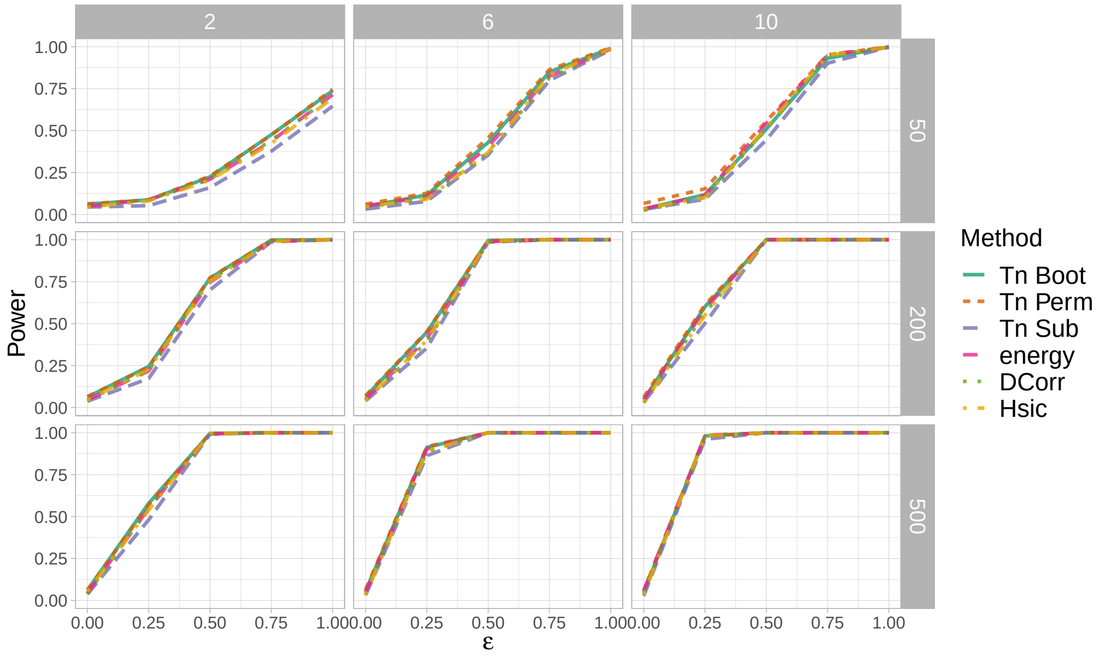


**Fig. S25** $t$-distribution: Power of KBQD test $T_n$, with the critical value computed using bootstrap, permutation and subsampling, compared with the available $k$-sample tests, as function of $\varepsilon$, with $\epsilon$ from 0 to 1, following **Type 1** (top) **Type 2** (bottom) alternatives. The sample size per group $n = 50, 200, 500$ and dimension $d = 2, 6, 10$, are indicated as headers. The number of samples is $k = 3$.

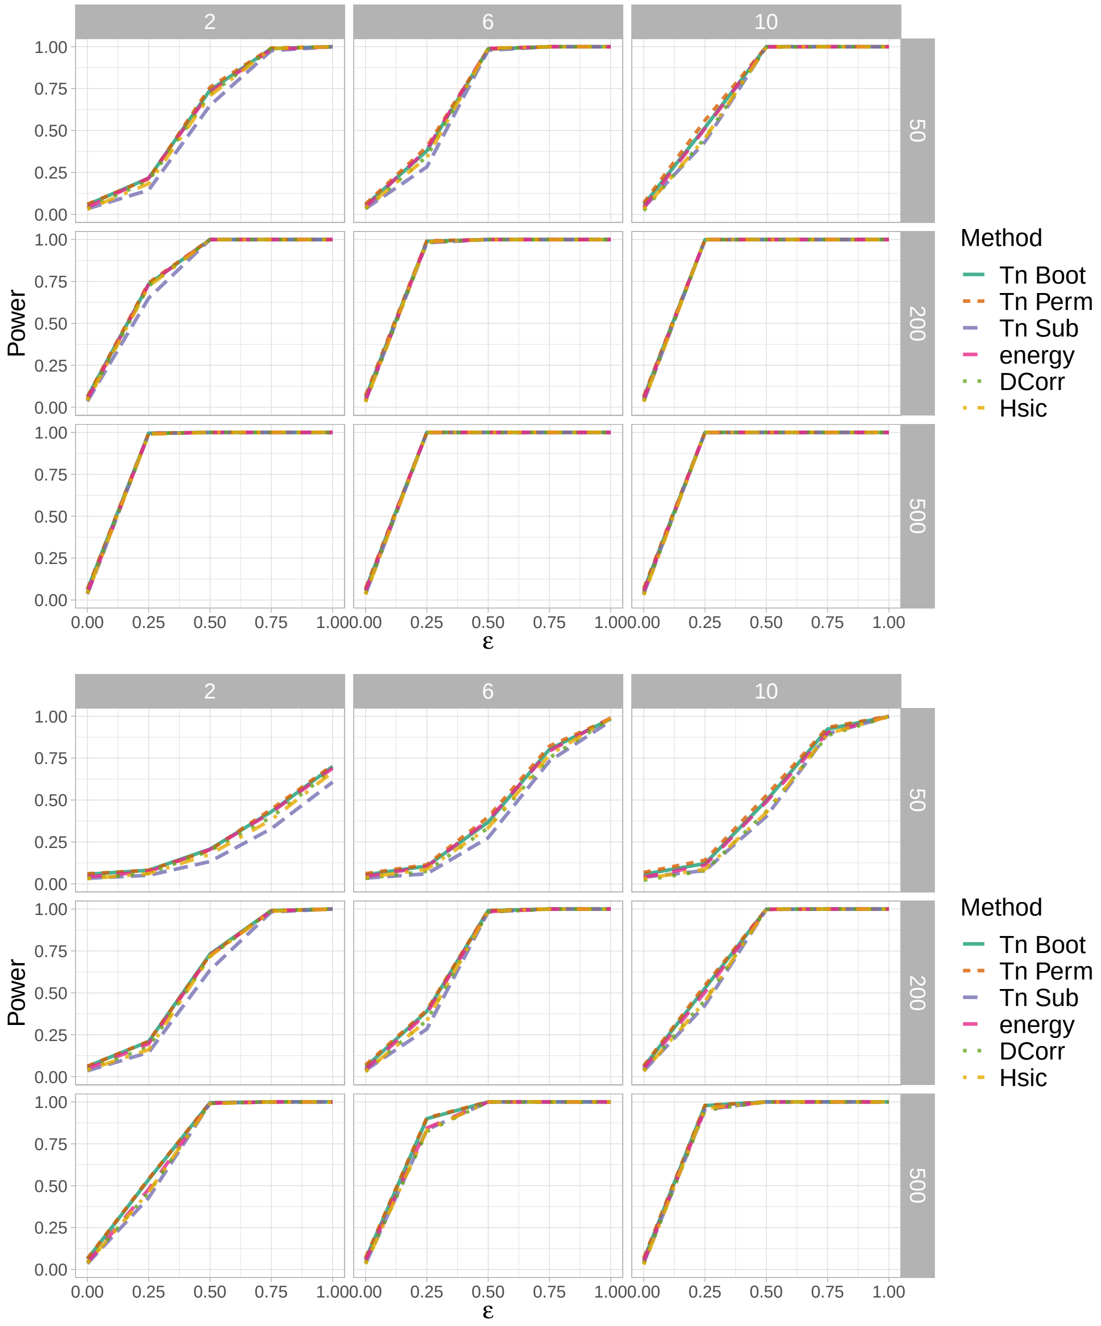


**Fig. S26** $t$-distribution: Power of KBQD test $T_n$, with the critical value computed using bootstrap, permutation and subsampling, compared with the available $k$-sample tests, as function of $\varepsilon$, with $\epsilon$ from 0 to 1, following **Type 1** (top) **Type 2** (bottom) alternatives. The sample size per group $n = 50, 200, 500$ and dimension $d = 2, 6, 10$, are indicated as headers. The number of samples is $k = 5$.
